# Supplementary material for: When Do LLMs Apply the Wrong Law? Diagnosing LLM Failures in Temporal Legal Reasoning
Source: arXiv:2608.14610 source file (2026-10-15)
Supplement: Supplementary file 2 [file TALD_appendix_preview.tex]

\documentclass[11pt]{article}
\usepackage[preprint]{acl}
\usepackage{times}
\usepackage[T1]{fontenc}
\usepackage[utf8]{inputenc}
\usepackage{amsmath,amssymb,booktabs,multirow}
\usepackage{array}
\usepackage{microtype}
\usepackage{placeins}
\IfFileExists{inconsolata.sty}{\usepackage{inconsolata}}{}
\input{env.tex}
\newcommand{\TALDMainRef}[1]{\ref*{#1}}
\input{others/TALD_main_references.tex}
\begin{document}
\appendix
\input{Sections/TALD_appendix_prefilled_v2}
\FloatBarrier
\bibliography{custom}
\end{document}
